# Supplementary material for: Intervals of permutation class growth rates
Source: arXiv:1410.3679 ancillary file (2015-09-03)
Supplement: Supplementary file 1 [file intervalCalculations.pdf]

# Calculating intervals of permutation class growth rates

David Bevan

This document is a copy of a *Mathematica* notebook containing the computer-aided calculations used in the proofs of the theorems in the article, "Intervals of permutation class growth rates" [<http://arxiv.org/pdf/1410.3679.pdf>]. It should be read in conjunction with that article.

The original *Mathematica* notebook is available from <http://arxiv.org/src/1410.3679/anc/intervalCalculations.nb>.

Section 1 consists of the *Mathematica* function definitions. Sections 2, 3 and 4 contain the calculations for the proof of Theorem 1, for Example 4.4, and for the proof of Theorem 2, respectively.

---

## I. *Mathematica* function definitions

### I.1 Utility functions

```
isSubsetOf::usage = "isSubsetOf[s,t] returns True
    if set s is a subset of set t, and False otherwise.";
isSubsetOf[s_, t_] := Complement[s, t] == {}
? isSubsetOf
```

isSubsetOf[s,t] returns True if set s is a subset of set t, and False otherwise.

```
colForm::usage = "colForm[s] prints list s in a column.";
colForm[s_] := (Print@Column@s; s;)
? colForm
tableForm::usage =
    "tableForm[k][s] displays s using TableForm with TableDepth set to k.";
tableForm[k_][s_] := TableForm[s, TableDepth -> k]
? tableForm
```

colForm[s] prints list s in a column.

tableForm[k][s] displays s using TableForm with TableDepth set to k.

## I.2 Functions relating to permutations

```

inflatePerm::usage =
  "inflatePerm[ $\sigma$ ,k,r] gives the permutation that results from
    inflating the kth entry of permutation  $\sigma$  with 1...r.";
inflatePerm[ $\sigma$ _, k_, r_] := Module[{e =  $\sigma$ [[k]]}, ReplacePart[
  If[# > e, # + r - 1, #] & /@  $\sigma$ , k → Sequence @@ Range[e, e + r - 1]]]
? inflatePerm
 $\omega$ Perm::usage =
  " $\omega$ Perm[n] gives the primary oscillation of length n.\n $\omega$ Perm[n,a,b]
    gives the primary oscillation of length n
    with the ends inflated with 1...a and 1...b.";
 $\omega$ Perm[1] = {1};
 $\omega$ Perm[2] = {2, 1};
 $\omega$ Perm[n_] :=
  Join[{3, 1}, Riffle[Range[5, n, 2], Range[2, n - 3, 2]], {n - 1}] /; OddQ[n]
 $\omega$ Perm[n_] :=
  Join[{3, 1}, Riffle[Range[5, n - 1, 2], Range[2, n - 4, 2]], {n, n - 2}] /; EvenQ[n]
 $\omega$ Perm[n_, a_, b_] := inflatePerm[inflatePerm[ $\omega$ Perm[n], n, b], 2, a] /; OddQ[n]
 $\omega$ Perm[n_, a_, b_] := inflatePerm[inflatePerm[ $\omega$ Perm[n], n - 1, b], 2, a] /; EvenQ[n]
?  $\omega$ Perm
 $\omega$ BarPerm::usage =
  " $\omega$ BarPerm[n] gives the secondary oscillation of length n.\n $\omega$ BarPerm[n,a,b]
    gives the secondary oscillation of length n
    with the ends inflated with 1...a and 1...b.";
 $\omega$ BarPerm[n_] := Delete[ $\omega$ Perm[n + 1], 2] - 1
 $\omega$ BarPerm[n_, a_, b_] := inflatePerm[Delete[ $\omega$ Perm[n + 1, 1, b], 2] - 1, 1, a]
?  $\omega$ BarPerm
 $\psi$ Perm::usage = " $\psi$ Perm[n] gives the star permutation {n+1,1,...,n}.";
 $\psi$ Perm[n_] := Join[{n + 1}, Range[n]]
?  $\psi$ Perm

```

$\text{inflatePerm}[\sigma, k, r]$  gives the permutation that results from inflating the  $k$ th entry of permutation  $\sigma$  with 1... $r$ .

$\omega$ Perm[n] gives the primary oscillation of length  $n$ .

$\omega$ Perm[n,a,b] gives the primary oscillation of length  $n$  with the ends inflated with 1... $a$  and 1... $b$ .

$\omega$ BarPerm[n] gives the secondary oscillation of length  $n$ .

$\omega$ BarPerm[n,a,b] gives the secondary oscillation of length  $n$  with the ends inflated with 1... $a$  and 1... $b$ .

$\psi$ Perm[n] gives the star permutation { $n+1, 1, \dots, n$ }.

```

coveredPerm[σ_, k_] := Module[{e = σ[[k]]}, If[# > e, #-1, #] & /@Delete[σ, k]]
coveredPerms[σ_] := DeleteDuplicates@Table[coveredPerm[σ, k], {k, Length@σ}]
subPerms::usage =
  "subPerms[σ] gives a list of the subpermutations of permutation σ.";
subPerms[σ_] := Join@@NestWhileList[
  DeleteDuplicates[Join@@coveredPerms /@#] &, {σ}, # ≠ {{1}} &]
? subPerms

```

subPerms[σ] gives a list of the subpermutations of permutation σ.

```

isIndecomposable::usage =
  "isIndecomposable[σ] returns True if permutation σ is
  sum indecomposable, and False otherwise.";
isIndecomposable[σ_] := And@@Most@Thread[FoldList[Max, σ] > Range@Length@σ]
? isIndecomposable
Clear@subIndecomposablesOfSet
subIndecomposablesOfSet::usage =
  "subIndecomposablesOfSet[s] gives a list of the
  indecomposable subpermutations of permutations in set s.";
subIndecomposablesOfSet[s_] := subIndecomposablesOfSet[s] =
  Select[DeleteDuplicates[Join@@subPerms /@ s], isIndecomposable]
? subIndecomposablesOfSet
Clear@isSubIndecomp
isSubIndecomp::usage =
  "isSubIndecomp[σ, τ] returns True if permutation σ is an
  indecomposable subpermutation of τ, and False otherwise.";
isSubIndecomp[σ_, τ_] := isSubIndecomp[s, t] =
  MemberQ[subIndecomposablesOfSet@{τ}, σ]
? isSubIndecomp

```

isIndecomposable[σ] returns True if permutation σ is sum indecomposable, and False otherwise.

subIndecomposablesOfSet[s] gives a list of the indecomposable subpermutations of permutations in set s.

isSubIndecomp[σ, τ] returns True if permutation σ is an indecomposable subpermutation of τ, and False otherwise.

```

permGraphEdges[σ_, k_] := Select[σ[[k+1 ;;]], σ[[k]] > # &]
permGraphEdges[σ_] :=
  Join@@Table[{{k, σ[[k]]}, {Position[σ, #][[1, 1], #]} & /@ permGraphEdges[σ, k],
    {k, 1, Length@σ - 1}]
showPerm::usage = "showPerm[σ] displays a plot
  of the (graph of) permutation σ.";
showPerm[σ_] := Show[
  ListPlot[σ, Axes → None, Frame → True, FrameTicks → None,
    AspectRatio → 1, PlotRange → {{0, Length@σ + 1}, {0, Length@σ + 1}},
    PlotStyle → Directive[PointSize[Medium], Darker@Blue], ImageSize → Tiny],
  Graphics[{Thin, Lighter@Gray, Line[permGraphEdges[σ]]}]]]
? showPerm
showPerms::usage = "showPerms[s] displays
  plots of the (graphs of) permutations in the list s.";
showPerms[s_] := Row[showPerm /@ s, "    "]
? showPerms

```

showPerm[σ] displays a plot of the (graph of) permutation  $\sigma$ .

showPerms[s] displays plots of the (graphs of) permutations in the list s.

### I.3 Functions relating to partial orders

```

maxElements::usage = "maxElements[s,p] gives a list
  of the maximal elements in s under the partial order p.";
maxElements[s_, p_] := accumMaxElements[{}, s, p]
accumMaxElements[r_, {}, _] := r
accumMaxElements[r_, {x_, xs___}, p_] := If[AnyTrue[r, p[x, #] &],
  accumMaxElements[r, {xs}, p], accumMaxElements[Join[r, {x}], {xs}, p]]
?maxElements
incomparable[x_, y_, p_] := incomparable[x, y, p] = ! (p[x, y] || p[y, x])
incomparable::usage =
  "incomparable[x,y,p] returns True if x and y are incomparable
  under partial order p, and False otherwise.";
?incomparable
incomparableSet[x_, s_, p_] := AllTrue[s, incomparable[x, #, p] &]
extendAntichain[a_, s_, p_] :=
  Join[a, {#}] & /@ Select[s, incomparableSet[#, a, p] &]
afterElement[s_, x_] := s[[Position[s, x, {1}, 1][[1, 1]] + 1 ;;]]
antichains[s_, p_] := Join[{{}}, Join@@
  NestWhileList[Join@@ (extendAntichain[#, afterElement[s, #[-1]], p] & /@ #) &,
  List /@ s, # != {} &]]
antichains::usage = "antichains[s,p] gives a list of all the
  antichains of elements of s under partial order p.";
?antichains
notGreaterThanAny[x_, s_, p_] :=
  notGreaterThanAny[x, s, p] = AllTrue[s, ! p[#, x] &]
notGreaterThanAny::usage =
  "notGreaterThanAny[x,s,p] returns True if x is not greater
  than any of the elements of s under partial order p.";
?notGreaterThanAny
downSetFromAntichain[a_, s_, p_] := Select[s, notGreaterThanAny[#, a, p] &]
downsets[s_, p_] := Sort[downSetFromAntichain[#, s, p] & /@ antichains[s, p]]
downsets[s_, t_, p_] := Select[downsets[s, p], isSubsetOf[t, #] &];
downsets::usage =
  "downsets[s,p] gives a list of all the downsets of elements of
  s under partial order p.\ndownsets[s,t,p] gives
  a list of those downsets of elements of s under
  partial order p that include all the elements of t.";
?downsets

```

`maxElements[s,p]` gives a list of the maximal elements in  $s$  under the partial order  $p$ .

`incomparable[x,y,p]` returns True if  $x$  and  $y$  are incomparable under partial order  $p$ , and False otherwise.

`antichains[s,p]` gives a list of all the antichains of elements of  $s$  under partial order  $p$ .

`notGreaterThanAny[x,s,p]` returns True if  $x$  is not greater than any of the elements of  $s$  under partial order  $p$ .

`downsets[s,p]` gives a list of all the downsets of elements of  $s$  under partial order  $p$ .

`downsets[s,t,p]` gives a list of those downsets of elements of  $s$  under partial order  $p$  that include all the elements of  $t$ .

## I.4 Functions relating to enumeration sequences

```
enumSeqFromLengths[s_] := enumSeqFromLengths[s] = BinCounts[s, {1, Max[s] + 1}]
enumSeq::usage =
  "enumSeq[s] gives the finite enumeration sequence (a list of the number
    of permutations of each length) for the list of permutations s.";
enumSeq[{}] = {0};
enumSeq[s_] := enumSeqFromLengths[Length/@s]
?enumSeq
```

`enumSeq[s]` gives the finite enumeration sequence (a list of the number of permutations of each length) for the list of permutations  $s$ .

```
makeRepeatingEnumSeq[s_] :=
  MapAt[OverBar, Drop[s, 1 - LengthWhile[Reverse@s, # == s[[-1]] &]], -1]
buildEnumSeq::usage =
  "buildEnumSeq[d,k] gives the infinite enumeration sequence
    equivalent to  $(0^{k+1}, d, 0, d, 0, \dots)$  for the generalised digit  $d$ .";
buildEnumSeq::alternating = "Generated sequence `1` is alternating.";
buildEnumSeq[d_, k_] := Module[{s = Join[ConstantArray[0, k + 1],
  Table[Sum[d[[j]], {j, i, 1, -2}], {i, Length@d}]}],
  If[s[[-1]] != s[[-2]], Message[buildEnumSeq::alternating, s];
  {}, makeRepeatingEnumSeq[s]]]
?buildEnumSeq
```

`buildEnumSeq[d,k]` gives the infinite enumeration sequence equivalent to  $(0^{k+1}, d, 0, d, 0, \dots)$  for the generalised digit  $d$ .

```

isFiniteEnumSeq[s_] := IntegerQ@Last@s
addEnumSeqs::usage =
  "addEnumSeqs[t,u] adds (finite or infinite) enumeration sequences t and u.";
addEnumSeqs[t_, u_] := Module[{len = Max[Length@t, Length@u]},
  PadRight[t, len] + PadRight[u, len]] /;
  isFiniteEnumSeq[t] && isFiniteEnumSeq[u]
addEnumSeqs[t_, u_] := Module[{len = Max[Length@t, Length@u]},
  makeRepeatingEnumSeq[PadRight[MapAt[First, t, -1], len, t[[-1, 1]]] +
  PadRight[MapAt[First, u, -1], len, u[[-1, 1]]]]] /;
  ! isFiniteEnumSeq[t] && ! isFiniteEnumSeq[u]
addEnumSeqs[t_, u_] := addEnumSeqs[Join[t, {OverBar@0}], u] /;
  isFiniteEnumSeq[t] && ! isFiniteEnumSeq[u]
addEnumSeqs[t_, u_] := addEnumSeqs[t, Join[u, {OverBar@0}]] /;
  ! isFiniteEnumSeq[t] && isFiniteEnumSeq[u]
? addEnumSeqs

```

addEnumSeqs[t,u] adds (finite or infinite) enumeration sequences t and u.

```

grSumClosed::usage =
  "grSumClosed[e] gives the growth rate of the sum-closed class whose
  indecomposables are enumerated by the sequence e. [Lemma 3.1]";
grSumClosed[e_] := Reduce[FromDigits[Reverse[Most@e], 1 /  $\gamma$ ] /  $\gamma$  +
  e[[-1, 1]]  $\gamma^{(1 - \text{Length}[e])} / (\gamma - 1) == 1$  &&  $\gamma > 1$ ,  $\gamma$ , Reals][[2]]
? grSumClosed

```

grSumClosed[e] gives the growth rate of the sum-closed class whose indecomposables are enumerated by the sequence e. [Lemma 3.1]

```

rootForm::usage = "rootForm[r] prints expression r
  containing a Root[e,n] object in a more readable form.";
rootForm[r_] := (Print[r /. Root[e_, n_] =>
  rootOf[MinimalPolynomial[Root[e, n], x]] // TraditionalForm];
  r;)
? rootForm

```

rootForm[r] prints expression r containing a Root[e,n] object in a more readable form.

## I.5 Functions relating to gap inequalities

```

smallerGap::usage =
  "smallerGap[a,b] yields True if a is determined to be a smaller
  gap than b assuming  $\gamma > 2$ , and False otherwise.";
smallerGap[a_, b_] := TrueQ[Simplify[a < b, Assumptions ->  $\gamma > 2$ ]]
? smallerGap

```

smallerGap[a,b] yields True if a is determined to be a smaller gap than b assuming  $\gamma > 2$ , and False otherwise.

```

gammaForm[e_] := Apart@FromDigits[Reverse@e, 1 /  $\gamma$ ]
bigDeltaRange::usage =
  "bigDeltaRange[dd] gives the big delta (range) value for
  the list of generalised digits dd.";
bigDeltaRange[dd_] := gammaForm@Last@dd - gammaForm@First@dd
?bigDeltaRange
maximalGaps::usage =
  "maximalGaps[dd] gives a list of the possibly maximal gaps between
  terms in the list of generalised digits dd, assuming  $\gamma > 2$ .";
maximalGaps[dd_] := maxElements[DeleteDuplicates@Differences[gammaForm /@ dd],
  smallerGap]
?maximalGaps

```

bigDeltaRange[dd] gives the big delta (range) value for the list of generalised digits dd.

maximalGaps[dd] gives a list of the possibly maximal gaps between terms in the list of generalised digits dd, assuming  $\gamma > 2$ .

```

gapInequality[ $\Delta$ _,  $\delta$ _] := Apart[( $\gamma^2 - 1$ )  $\delta$ ]  $\leq \Delta$ 
gapInequality[ $\Delta$ _,  $\delta$ _, k_] := Apart[( $\gamma^{k-1} - \gamma^{k-3}$ )  $\delta$ ]  $\leq \Delta$ 
gapInequalities::usage =
  "gapInequalities[dd] gives a list of the gap inequalities
  for the sequence of sets of generalised digits ( $D_n$ ), where
   $D_n = dd$  for every sufficiently large odd  $n$  and  $D_n = \{0\}$ 
  otherwise. \ngapInequalities[dd1, dd, k] gives a list of the
  gap inequalities for the sequence of sets of generalised
  digits ( $D_n$ ), where  $D_1 = dd_1$ ,  $D_n = dd$  for every odd  $n \geq k$ 
  ( $k \geq 3$  odd), and  $D_n = \{0\}$  otherwise. \n[Corollary 2.3]";
gapInequalities[dd_] := gapInequality[bigDeltaRange[dd], #] & /@ maximalGaps[dd]
gapInequalities[dd1_, dd_, k_] :=
  Join[gapInequality[bigDeltaRange[dd], #] & /@ maximalGaps[dd],
  gapInequality[bigDeltaRange[dd], #, k] & /@ maximalGaps[dd1]]
?gapInequalities

```

gapInequalities[dd] gives a list of the gap inequalities for the sequence of sets of generalised digits ( $D_n$ ), where  $D_n = dd$  for every sufficiently large odd  $n$  and  $D_n = \{0\}$  otherwise.

gapInequalities[dd<sub>1</sub>, dd, k] gives a list of the gap inequalities for the sequence of sets of generalised digits ( $D_n$ ), where  $D_1 = dd_1$ ,  $D_n = dd$  for every odd  $n \geq k$  ( $k \geq 3$  odd), and  $D_n = \{0\}$  otherwise.

[Corollary  
2.3]

```

orderGammaSums[e_] := HoldForm /@ Evaluate[e /. Plus -> plus /.
  plus[s_] := plus @@ SortBy[{s}, -Abs[#] /.  $\gamma \rightarrow 1000$  &]] /. plus -> Plus
gapIneqsForm::usage = "gapIneqsForm[e] prints the list of
  inequalities e as a vertical list with powers displayed
  as superscripts and terms in sums ordered appropriately.";
gapIneqsForm[e_] := (Print[tableForm[1][orderGammaSums@e] /.
  Power[a_, b_] := SuperscriptBox[a, b] // DisplayForm];
  e);
? gapIneqsForm

```

gapIneqsForm[e] prints the list of inequalities e as a vertical list with powers displayed as superscripts and terms in sums ordered appropriately.

## I.6 Functions relating to the interval constructions

```

columnMaximaSeqsForF[r_, s_, i_, j_] :=
  Join[ConstantArray[r, i], Reverse@#] & /@ Subsets[Range[2, r - 1], {s - i - j - 1}]
columnMaximaSeqsForF[r_, s_] :=
  Flatten[Table[columnMaximaSeqsForF[r, s, i, j], {i, 0, s - 1}, {j, 0, s - i - 1}], 2]
downsetFromColumnMaximaSeqForF[maxList_] :=
  Join @@ MapIndexed[Table[{k, #2[[1]] + 1}, {k, 2, #}], maxList]
enumerateDownsetForF[s_] := Rest[BinCounts[Total /@ s]]
sortEnumerations::usage = "sortEnumerations[ee]
  sorts list of enumerations ee in lexicographic order.";
sortEnumerations[ee_] := SortBy[ee, PadRight[#, Max[Length /@ ee]] &]
? sortEnumerations
enumerationsForF::usage =
  "enumerationsForF[r, s] gives a list of the distinct enumerations
  of downsets in  $\mathcal{F}^{r,s}$ . [Lemma 4.2].";
enumerationsForF[r_, s_] := sortEnumerations[enumerateDownsetForF /@
  downsetFromColumnMaximaSeqForF /@ columnMaximaSeqsForF[r, s]] [[3 ;;]]
? enumerationsForF

```

sortEnumerations[ee] sorts list of enumerations ee in lexicographic order.

enumerationsForF[r,s] gives a list of the distinct enumerations of downsets in  $\mathcal{F}^{r,s}$ . [Lemma 4.2].

```

countQ::usage =
  "countQ[r, s] gives the infinite enumeration sequence of the set
  of indecomposables  $Q^{r,s}$ . [Lemma 4.3]";
countQ[r_, s_] := countQ[s, r] /; r < s
countQ[r_, r_] := Join[{1, 1, 2}, Range[3, 2 r - 1, 2], {OverBar[2 r]}]
countQ[r_, s_] :=
  makeRepeatingEnumSeq[Join[{1, 1, 2}, Range[3, 2 s + 1, 2], Range[2 s + 2, r + s]]]
? countQ

```

countQ[r,s] gives the infinite enumeration sequence of the set of indecomposables  $Q^{r,s}$ . [Lemma 4.3]

```

qSetPerms::usage =
  "qSetPerms[r,s,n] gives the set of indecomposables in  $Q^{r,s}$  of
  length at most n. [Lemma 4.3]";
qSetPerms[r_, s_, n_] := qSetPerms[s, r, n] /; r < s
qSetPerms[r_, s_, n_] := Sort@Join[
  Table[ $\omega$ Perm[m], {m, n}],
  Table[ $\omega$ BarPerm[m], {m, 3, n}],
  Table[ $\psi$ Perm[u], {u, 3, Min[r+1, n-1]}],
  Join@@Table[ $\omega$ Perm[m, u, 1], {m, 4, n-1}, {u, 2, Min[r, n+1-m]}],
  Join@@Table[ $\omega$ Perm[m, 1, v], {m, 5, n-1, 2}, {v, 2, Min[s, n+1-m]}],
  Join@@Table[ $\omega$ BarPerm[m, 1, v], {m, 4, n-1, 2}, {v, 2, Min[s, n+1-m]}]]
? qSetPerms

```

qSetPerms[r,s,n] gives the set of indecomposables in  $Q^{r,s}$  of length at most n. [Lemma 4.3]

## 2. Calculations for the proof of Theorem I

```

q53Seq = countQ[5, 3]
grSumClosed@% // rootForm
N[%, 7]
{1, 1, 2, 3, 5, 7,  $\overline{8}$ }
rootOf( $x^7 - 2x^6 - x^4 - x^3 - 2x^2 - 2x - 1$ )
2.355257

f53Seqs = enumerationsForF[5, 3]
Table[addEnumSeqs[q53Seq, buildEnumSeq[First@f53Seqs, k]], {k, 5, 11, 2}] //
  tableForm@1
Table[addEnumSeqs[q53Seq, buildEnumSeq[Last@f53Seqs, k]], {k, 5, 11, 2}] //
  tableForm@1
grSumClosed@[1] // rootForm
N[%, 7]
{{1, 1}, {1, 1, 1}, {1, 1, 1, 1}, {1, 2}, {1, 2, 1},
 {1, 2, 1, 1}, {1, 2, 2}, {1, 2, 2, 1}, {1, 2, 2, 2}, {1, 2, 2, 2, 1}}
{1, 1, 2, 3, 5, 7,  $\overline{9}$ }
{1, 1, 2, 3, 5, 7, 8, 8,  $\overline{9}$ }
{1, 1, 2, 3, 5, 7, 8, 8, 8, 8,  $\overline{9}$ }
{1, 1, 2, 3, 5, 7, 8, 8, 8, 8, 8, 8,  $\overline{9}$ }
{1, 1, 2, 3, 5, 7, 9, 10, 11,  $\overline{12}$ }
{1, 1, 2, 3, 5, 7, 8, 8, 9, 10, 11,  $\overline{12}$ }
{1, 1, 2, 3, 5, 7, 8, 8, 8, 8, 9, 10, 11,  $\overline{12}$ }
{1, 1, 2, 3, 5, 7, 8, 8, 8, 8, 8, 8, 9, 10, 11,  $\overline{12}$ }
rootOf( $x^{10} - 2x^9 - x^7 - x^6 - 2x^5 - 2x^4 - 2x^3 - x^2 - x - 1$ )
2.362008

```

```

gapInequalities@f53Seqs // gapIneqsForm
Reduce[And@@% &&  $\gamma > 1$ ,  $\gamma$ ] // rootForm
N[%[[3 ;;]], 7]
 $1 - \gamma^{-2} \leq \gamma^{-1} + 2\gamma^{-2} + 2\gamma^{-3} + \gamma^{-4}$ 
 $\gamma - 1 - 2\gamma^{-1} + \gamma^{-2} + \gamma^{-3} \leq \gamma^{-1} + 2\gamma^{-2} + 2\gamma^{-3} + \gamma^{-4}$ 
 $1 < \gamma \leq \text{rootOf}(x^4 - 2x^3 - x^2 - 1)$ 
 $\gamma \leq 2.470979$ 

```

### 3. Calculations for Example 4.4

```

hSet = Complement[subIndecomposablesOfSet@{ $\omega$ Perm[5, 7, 1]}, qSetPerms[5, 3, 10]];
showPerms@hSet

```

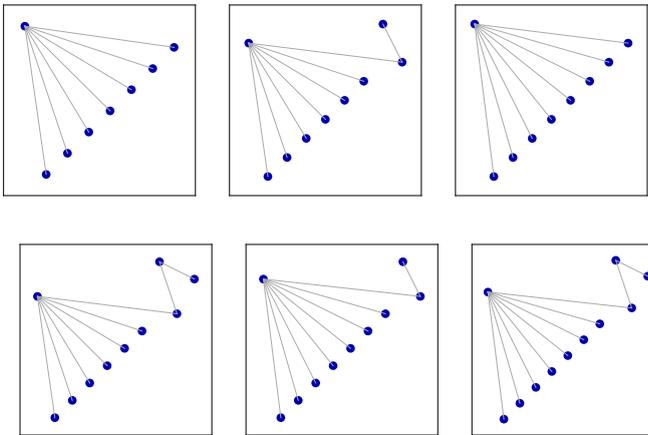

```

q53Seq = countQ[5, 3]
f53Seqs = enumerationsForF[5, 3]
Length@%
downsets[hSet, {ψPerm[7]}, isSubIndecomp]
hSeqs = sortEnumerations@DeleteDuplicates[enumSeq/@%]
Length@%
addEnumSeqs[addEnumSeqs[q53Seq, buildEnumSeq[First@f53Seqs, 5]], First@hSeqs]
grSumClosed@% // rootForm
N[%, 7]
addEnumSeqs[addEnumSeqs[q53Seq, buildEnumSeq[Last@f53Seqs, 5]], Last@hSeqs]
grSumClosed@% // rootForm
N[%, 7]
{1, 1, 2, 3, 5, 7, 8̄}

{{1, 1}, {1, 1, 1}, {1, 1, 1, 1}, {1, 2}, {1, 2, 1},
 {1, 2, 1, 1}, {1, 2, 2}, {1, 2, 2, 1}, {1, 2, 2, 2}, {1, 2, 2, 2, 1}}

10
{{{8, 1, 2, 3, 4, 5, 6, 7}}, {{8, 1, 2, 3, 4, 5, 6, 7}, {8, 1, 2, 3, 4, 5, 6, 9, 7}},
 {{8, 1, 2, 3, 4, 5, 6, 7}, {9, 1, 2, 3, 4, 5, 6, 7, 8}},
 {{8, 1, 2, 3, 4, 5, 6, 7}, {8, 1, 2, 3, 4, 5, 6, 9, 7}, {9, 1, 2, 3, 4, 5, 6, 7, 8}},
 {{8, 1, 2, 3, 4, 5, 6, 7}, {8, 1, 2, 3, 4, 5, 6, 9, 7}, {8, 1, 2, 3, 4, 5, 6, 10, 7, 9}},
 {{8, 1, 2, 3, 4, 5, 6, 7}, {8, 1, 2, 3, 4, 5, 6, 9, 7}, {9, 1, 2, 3, 4, 5, 6, 7, 8},
 {8, 1, 2, 3, 4, 5, 6, 10, 7, 9}}, {{8, 1, 2, 3, 4, 5, 6, 7}, {8, 1, 2, 3, 4, 5, 6, 9, 7},
 {9, 1, 2, 3, 4, 5, 6, 7, 8}, {9, 1, 2, 3, 4, 5, 6, 7, 10, 8}},
 {{8, 1, 2, 3, 4, 5, 6, 7}, {8, 1, 2, 3, 4, 5, 6, 9, 7}, {9, 1, 2, 3, 4, 5, 6, 7, 8},
 {8, 1, 2, 3, 4, 5, 6, 10, 7, 9}, {9, 1, 2, 3, 4, 5, 6, 7, 10, 8}},
 {{8, 1, 2, 3, 4, 5, 6, 7}, {8, 1, 2, 3, 4, 5, 6, 9, 7},
 {9, 1, 2, 3, 4, 5, 6, 7, 8}, {8, 1, 2, 3, 4, 5, 6, 10, 7, 9},
 {9, 1, 2, 3, 4, 5, 6, 7, 10, 8}, {9, 1, 2, 3, 4, 5, 6, 7, 11, 8, 10}}}

{{0, 0, 0, 0, 0, 0, 0, 0, 1}, {0, 0, 0, 0, 0, 0, 0, 0, 1, 1}, {0, 0, 0, 0, 0, 0, 0, 0, 1, 1, 1},
 {0, 0, 0, 0, 0, 0, 0, 0, 1, 2}, {0, 0, 0, 0, 0, 0, 0, 0, 1, 2, 1},
 {0, 0, 0, 0, 0, 0, 0, 0, 1, 2, 2}, {0, 0, 0, 0, 0, 0, 0, 0, 1, 2, 2, 1}}

7
{1, 1, 2, 3, 5, 7, 9, 10, 9̄}

rootOf(x9 - 2 x8 - x6 - x5 - 2 x4 - 2 x3 - 2 x2 - x + 1)
2.360281

{1, 1, 2, 3, 5, 7, 9, 11, 13, 14, 13, 12̄}

rootOf(x12 - 2 x11 - x9 - x8 - 2 x7 - 2 x6 - 2 x5 - 2 x4 - 2 x3 - x2 + x + 1)
2.364197

gapInequalities[hSeqs, f53Seqs, 7] // gapIneqsForm
Reduce[And@@% && γ > 1, γ] // rootForm
N[%[[3 ;;], 7]

```

$$1 - \gamma^{-2} \leq \gamma^{-1} + 2\gamma^{-2} + 2\gamma^{-3} + \gamma^{-4}$$

$$\gamma - 1 - 2\gamma^{-1} + \gamma^{-2} + \gamma^{-3} \leq \gamma^{-1} + 2\gamma^{-2} + 2\gamma^{-3} + \gamma^{-4}$$

$$\gamma^{-2} - \gamma^{-4} \leq \gamma^{-1} + 2\gamma^{-2} + 2\gamma^{-3} + \gamma^{-4}$$

$$1 < \gamma \leq \text{rootOf}(x^4 - 2x^3 - x^2 - 1)$$

$$\gamma \leq 2.470979$$

## 4. Calculations for the proof of Theorem 2

### 4.1 Family A

```

π1 = ωPerm[7, 9, 1];
μ1 = ψPerm[7];
aSet = Complement[subIndecomposablesOfSet@{π1}, qSetPerms[5, 3, 14]];
showPerms@aSet

```

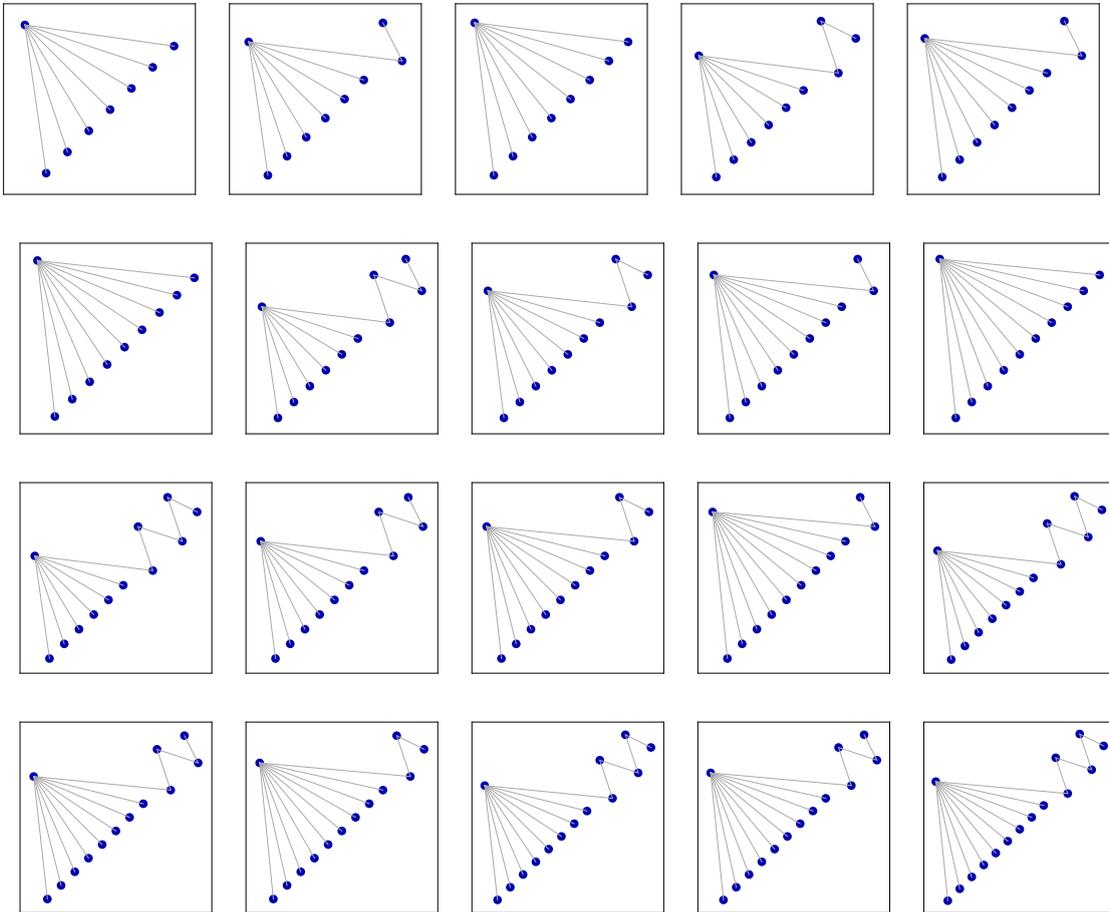

```

q53Seq = countQ[5, 3]
f53Seqs = enumerationsForF[5, 3]
Length@%
downsets[aSet, {μ1}, isSubIndecomp];
aSeqs = sortEnumerations@DeleteDuplicates[enumSeq/@%]
Length@%
addEnumSeqs[addEnumSeqs[q53Seq, buildEnumSeq[First@f53Seqs, 7]], First@aSeqs]
grSumClosed@% // rootForm
N[%, 7]
addEnumSeqs[addEnumSeqs[q53Seq, buildEnumSeq[Last@f53Seqs, 7]], Last@aSeqs]
grSumClosed@% // rootForm
N[%, 7]
{1, 1, 2, 3, 5, 7, 8}
{{1, 1}, {1, 1, 1}, {1, 1, 1, 1}, {1, 2}, {1, 2, 1},
  {1, 2, 1, 1}, {1, 2, 2}, {1, 2, 2, 1}, {1, 2, 2, 2}, {1, 2, 2, 2, 1}}
10
{{0, 0, 0, 0, 0, 0, 0, 0, 1}, {0, 0, 0, 0, 0, 0, 0, 0, 1, 1}, {0, 0, 0, 0, 0, 0, 0, 0, 1, 1, 1},
  {0, 0, 0, 0, 0, 0, 0, 0, 1, 1, 1, 1}, {0, 0, 0, 0, 0, 0, 0, 0, 1, 1, 1, 1, 1},
  {0, 0, 0, 0, 0, 0, 0, 0, 1, 2}, {0, 0, 0, 0, 0, 0, 0, 0, 1, 2, 1},
  {0, 0, 0, 0, 0, 0, 0, 0, 1, 2, 1, 1}, {0, 0, 0, 0, 0, 0, 0, 0, 1, 2, 1, 1, 1},
  {0, 0, 0, 0, 0, 0, 0, 0, 1, 2, 2}, {0, 0, 0, 0, 0, 0, 0, 0, 1, 2, 2, 1},
  {0, 0, 0, 0, 0, 0, 0, 0, 1, 2, 2, 1, 1}, {0, 0, 0, 0, 0, 0, 0, 0, 1, 2, 2, 2},
  {0, 0, 0, 0, 0, 0, 0, 0, 1, 2, 2, 2, 1}, {0, 0, 0, 0, 0, 0, 0, 0, 1, 2, 2, 2, 2},
  {0, 0, 0, 0, 0, 0, 0, 0, 1, 2, 2, 2, 2, 1}, {0, 0, 0, 0, 0, 0, 0, 0, 1, 2, 3},
  {0, 0, 0, 0, 0, 0, 0, 0, 1, 2, 3, 1}, {0, 0, 0, 0, 0, 0, 0, 0, 1, 2, 3, 1, 1},
  {0, 0, 0, 0, 0, 0, 0, 0, 1, 2, 3, 2}, {0, 0, 0, 0, 0, 0, 0, 0, 1, 2, 3, 2, 1},
  {0, 0, 0, 0, 0, 0, 0, 0, 1, 2, 3, 2, 2}, {0, 0, 0, 0, 0, 0, 0, 0, 1, 2, 3, 2, 2, 1},
  {0, 0, 0, 0, 0, 0, 0, 0, 1, 2, 3, 3}, {0, 0, 0, 0, 0, 0, 0, 0, 1, 2, 3, 3, 1},
  {0, 0, 0, 0, 0, 0, 0, 0, 1, 2, 3, 3, 2}, {0, 0, 0, 0, 0, 0, 0, 0, 1, 2, 3, 3, 2, 1},
  {0, 0, 0, 0, 0, 0, 0, 0, 1, 2, 3, 3, 3}, {0, 0, 0, 0, 0, 0, 0, 0, 1, 2, 3, 3, 3, 1},
  {0, 0, 0, 0, 0, 0, 0, 0, 1, 2, 3, 3, 3, 2}, {0, 0, 0, 0, 0, 0, 0, 0, 1, 2, 3, 3, 3, 2, 1},
  {0, 0, 0, 0, 0, 0, 0, 0, 1, 2, 3, 4}, {0, 0, 0, 0, 0, 0, 0, 0, 1, 2, 3, 4, 1},
  {0, 0, 0, 0, 0, 0, 0, 0, 1, 2, 3, 4, 2}, {0, 0, 0, 0, 0, 0, 0, 0, 1, 2, 3, 4, 2, 1},
  {0, 0, 0, 0, 0, 0, 0, 0, 1, 2, 3, 4, 3}, {0, 0, 0, 0, 0, 0, 0, 0, 1, 2, 3, 4, 3, 1},
  {0, 0, 0, 0, 0, 0, 0, 0, 1, 2, 3, 4, 3, 2}, {0, 0, 0, 0, 0, 0, 0, 0, 1, 2, 3, 4, 3, 2, 1},
  {0, 0, 0, 0, 0, 0, 0, 0, 1, 2, 3, 4, 4}, {0, 0, 0, 0, 0, 0, 0, 0, 1, 2, 3, 4, 4, 1},
  {0, 0, 0, 0, 0, 0, 0, 0, 1, 2, 3, 4, 4, 2}, {0, 0, 0, 0, 0, 0, 0, 0, 1, 2, 3, 4, 4, 2, 1},
  {0, 0, 0, 0, 0, 0, 0, 0, 1, 2, 3, 4, 4, 3}, {0, 0, 0, 0, 0, 0, 0, 0, 1, 2, 3, 4, 4, 3, 1},
  {0, 0, 0, 0, 0, 0, 0, 0, 1, 2, 3, 4, 4, 3, 2}, {0, 0, 0, 0, 0, 0, 0, 0, 1, 2, 3, 4, 4, 3, 2, 1}}

```

47

```

{1, 1, 2, 3, 5, 7, 8, 9}
rootOf(x^8 - 2 x^7 - x^5 - x^4 - 2 x^3 - 2 x^2 - x - 1)
2.356983
{1, 1, 2, 3, 5, 7, 8, 9, 11, 13, 15, 16, 15, 14, 13, 12}
rootOf(x^14 - 3 x^13 + 2 x^12 - 3 x^10 + x^9 - 2 x^7 + x^6 - x^5 - 2 x^4 + x^3 + 1)
2.359320

```

```

gapInequalities[aSeqs, f53Seqs, 9] // gapIneqsForm
Reduce[And@@% &&  $\gamma > 1$ ,  $\gamma$ ] // rootForm
N[%[[3 ;;], 7]
 $1 - \gamma^{-2} \leq \gamma^{-1} + 2\gamma^{-2} + 2\gamma^{-3} + \gamma^{-4}$ 
 $\gamma - 1 - 2\gamma^{-1} + \gamma^{-2} + \gamma^{-3} \leq \gamma^{-1} + 2\gamma^{-2} + 2\gamma^{-3} + \gamma^{-4}$ 
 $1 - \gamma^{-2} \leq \gamma^{-1} + 2\gamma^{-2} + 2\gamma^{-3} + \gamma^{-4}$ 
 $1 < \gamma \leq \text{rootOf}(x^4 - 2x^3 - x^2 - 1)$ 
 $\gamma \leq 2.470979$ 

```

## 4.2 Family B

```

 $\pi_2 = \{2, 9, 1, 3, 4, 5, 6, 7, 10, 8\}$ ;
bSet = Complement[subIndecomposablesOfSet@{ $\pi_2$ }, qSetPerms[5, 3, 10]];
showPerms@bSet

```

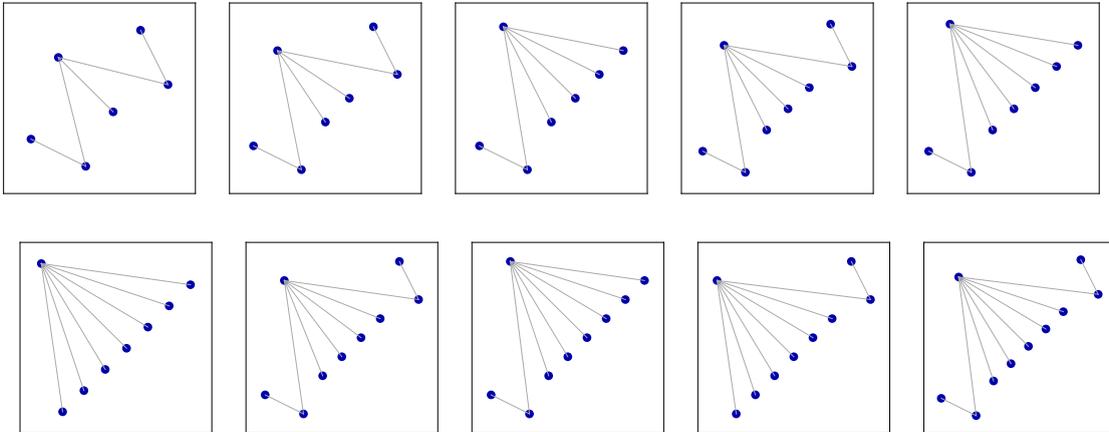

```

q53Seq = countQ[5, 3]
f53Seqs = enumerationsForF[5, 3]
Length@%
downsets[bSet, isSubIndecomp];
bSeqs = sortEnumerations@DeleteDuplicates[enumSeq / @%]
Length@%
addEnumSeqs[addEnumSeqs[q53Seq, buildEnumSeq[First@f53Seqs, 5]], First@bSeqs]
grSumClosed@% // rootForm
N[%, 7]
addEnumSeqs[addEnumSeqs[q53Seq, buildEnumSeq[Last@f53Seqs, 5]], Last@bSeqs]
grSumClosed@% // rootForm
N[%, 7]
{1, 1, 2, 3, 5, 7,  $\bar{8}$ }
{{1, 1}, {1, 1, 1}, {1, 1, 1, 1}, {1, 2}, {1, 2, 1},
{1, 2, 1, 1}, {1, 2, 2}, {1, 2, 2, 1}, {1, 2, 2, 2}, {1, 2, 2, 2, 1}}
10
{{0}, {0, 0, 0, 0, 0, 0, 0, 1}, {0, 0, 0, 0, 0, 0, 0, 1, 1},
{0, 0, 0, 0, 0, 0, 1}, {0, 0, 0, 0, 0, 0, 1, 1}, {0, 0, 0, 0, 0, 0, 1, 1, 1},
{0, 0, 0, 0, 0, 0, 1, 2}, {0, 0, 0, 0, 0, 0, 1, 2, 1}, {0, 0, 0, 0, 0, 0, 1, 2, 2},
{0, 0, 0, 0, 0, 1}, {0, 0, 0, 0, 0, 1, 0, 1}, {0, 0, 0, 0, 0, 1, 0, 1, 1},
{0, 0, 0, 0, 0, 1, 1}, {0, 0, 0, 0, 0, 1, 1, 1}, {0, 0, 0, 0, 0, 1, 1, 1, 1},
{0, 0, 0, 0, 0, 1, 1, 2}, {0, 0, 0, 0, 0, 1, 1, 2, 1}, {0, 0, 0, 0, 0, 1, 1, 2, 2},
{0, 0, 0, 0, 0, 1, 2}, {0, 0, 0, 0, 0, 1, 2, 1}, {0, 0, 0, 0, 0, 1, 2, 1, 1},
{0, 0, 0, 0, 0, 1, 2, 2}, {0, 0, 0, 0, 0, 1, 2, 2, 1}, {0, 0, 0, 0, 0, 1, 2, 2, 2},
{0, 0, 0, 0, 0, 1, 2, 3}, {0, 0, 0, 0, 0, 1, 2, 3, 1}, {0, 0, 0, 0, 0, 1, 2, 3, 2},
{0, 0, 0, 0, 0, 1, 2, 3, 3}, {0, 0, 0, 0, 0, 1, 2, 3, 3, 1}}
29
{1, 1, 2, 3, 5, 7,  $\bar{9}$ }
rootOf( $x^3 - 2x^2 - 2$ )
2.359304
{1, 1, 2, 3, 5, 8, 11, 13, 14, 13,  $\bar{12}$ }
rootOf( $x^{11} - 2x^{10} - x^8 - x^7 - 2x^6 - 3x^5 - 3x^4 - 2x^3 - x^2 + x + 1$ )
2.375872
gapInequalities[bSeqs, f53Seqs, 7] // gapIneqsForm
Reduce[And@@% &&  $\gamma > 1$ ,  $\gamma$ ] // rootForm
N[%[[3 ;;], 7]
 $1 - \gamma^{-2} \leq \gamma^{-1} + 2\gamma^{-2} + 2\gamma^{-3} + \gamma^{-4}$ 
 $\gamma - 1 - 2\gamma^{-1} + \gamma^{-2} + \gamma^{-3} \leq \gamma^{-1} + 2\gamma^{-2} + 2\gamma^{-3} + \gamma^{-4}$ 
 $\gamma^{-1} - \gamma^{-3} \leq \gamma^{-1} + 2\gamma^{-2} + 2\gamma^{-3} + \gamma^{-4}$ 
 $1 - \gamma^{-1} - 2\gamma^{-2} + \gamma^{-3} + \gamma^{-4} \leq \gamma^{-1} + 2\gamma^{-2} + 2\gamma^{-3} + \gamma^{-4}$ 
 $\gamma - 1 - 3\gamma^{-1} - \gamma^{-2} + 2\gamma^{-3} + 2\gamma^{-4} \leq \gamma^{-1} + 2\gamma^{-2} + 2\gamma^{-3} + \gamma^{-4}$ 
 $1 < \gamma \leq \text{rootOf}(x^4 - 2x^3 - x^2 - 1)$ 
 $\gamma \leq 2.470979$ 

```

## 4.3 Family C

```
 $\pi_3 = \{3, 1, 8, 2, 4, 5, 6, 10, 7, 9\};$ 
```

```
 $\mu_2 = \{2, 5, 1, 3, 6, 4\};$ 
```

```
cSet = Complement[subIndecomposablesOfSet@{ $\pi_3$ }, qSetPerms[9, 8, 10]];
```

```
showPerms@cSet
```

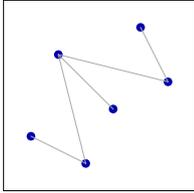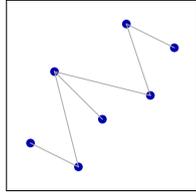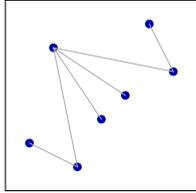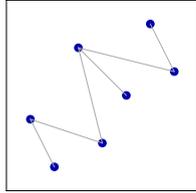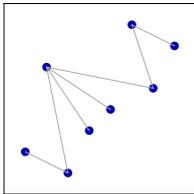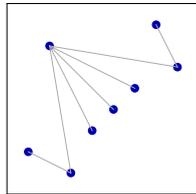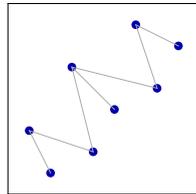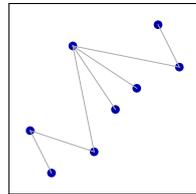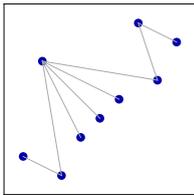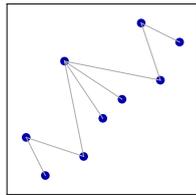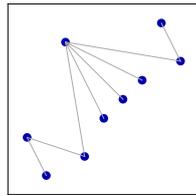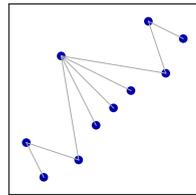

```

q98Seq = countQ[9, 8]
f98Seqs = enumerationsForF[9, 8];
Length@%
First@f98Seqs
Last@f98Seqs
downsets[cSet, {μ2}, isSubIndecomp];
cSeqs = sortEnumerations@DeleteDuplicates[enumSeq /@ %]
Length@%
addEnumSeqs[addEnumSeqs[q98Seq, buildEnumSeq[First@f98Seqs, 5]], First@cSeqs]
grSumClosed@% // rootForm
N[%, 7]
addEnumSeqs[addEnumSeqs[q98Seq, buildEnumSeq[Last@f98Seqs, 5]], Last@cSeqs]
grSumClosed@% // rootForm
N[%, 7]
{1, 1, 2, 3, 5, 7, 9, 11, 13, 15,  $\overline{17}$ }
574
{1, 1}
{1, 2, 3, 4, 5, 6, 7, 7, 6, 5, 4, 3, 2, 1}
{{0, 0, 0, 0, 0, 1}, {0, 0, 0, 0, 0, 1, 1}, {0, 0, 0, 0, 0, 1, 1, 1},
{0, 0, 0, 0, 0, 1, 2}, {0, 0, 0, 0, 0, 1, 2, 1}, {0, 0, 0, 0, 0, 1, 2, 2},
{0, 0, 0, 0, 0, 1, 2, 2, 1}, {0, 0, 0, 0, 0, 1, 3}, {0, 0, 0, 0, 0, 1, 3, 1},
{0, 0, 0, 0, 0, 1, 3, 2}, {0, 0, 0, 0, 0, 1, 3, 2, 1}, {0, 0, 0, 0, 0, 1, 3, 3},
{0, 0, 0, 0, 0, 1, 3, 3, 1}, {0, 0, 0, 0, 0, 1, 3, 3, 2},
{0, 0, 0, 0, 0, 1, 3, 4}, {0, 0, 0, 0, 0, 1, 3, 4, 1}, {0, 0, 0, 0, 0, 1, 3, 4, 2},
{0, 0, 0, 0, 0, 1, 3, 4, 3}, {0, 0, 0, 0, 0, 1, 3, 4, 3, 1}}
19
{1, 1, 2, 3, 5, 8, 10, 12, 14, 16,  $\overline{18}$ }
rootOf(x11 - 2 x10 - x8 - x7 - 2 x6 - 3 x5 - 2 x4 - 2 x3 - 2 x2 - 2 x - 2)
2.373983
{1, 1, 2, 3, 5, 8, 13, 17, 20, 22, 26, 29, 33, 36, 39, 41, 43, 44,  $\overline{45}$ }
rootOf(x19 - 2 x18 - x16 - x15 - 2 x14 - 3 x13 - 5 x12 -
4 x11 - 3 x10 - 2 x9 - 4 x8 - 3 x7 - 4 x6 - 3 x5 - 3 x4 - 2 x3 - 2 x2 - x - 1)
2.389043
gapInequalities[cSeqs, f98Seqs, 7] // gapIneqsForm
Reduce[And@@% && γ > 1, γ] // rootForm
N[%[[3 ;;], 7]
1 - γ-2 ≤ γ-1 + 3 γ-2 + 4 γ-3 + 5 γ-4 + 6 γ-5 + 7 γ-6 + 7 γ-7 + 6 γ-8 + 5 γ-9 + 4 γ-10 + 3 γ-11 + 2 γ-12 + γ-13
γ - 1 - 2 γ-1 + γ-6 + γ-7 ≤ γ-1 + 3 γ-2 + 4 γ-3 + 5 γ-4 + 6 γ-5 + 7 γ-6 + 7 γ-7 + 6 γ-8 + 5 γ-9 + 4 γ-10 + 3 γ-11 + 2 γ-12
1 - γ-2 ≤ γ-1 + 3 γ-2 + 4 γ-3 + 5 γ-4 + 6 γ-5 + 7 γ-6 + 7 γ-7 + 6 γ-8 + 5 γ-9 + 4 γ-10 + 3 γ-11 + 2 γ-12 + γ-13
1 < γ ≤ rootOf(x13 - 2 x12 - x11 - 2 x10 - 2 x9 - 3 x8 - 3 x7 - 3 x6 - 3 x5 - 3 x4 - 2 x3 - 2 x2 - x - 1)
γ ≤ 2.786389

```

## 4.4 Family D

```

π4 = {3, 1, 4, 5, 6, 2};
π5 = {2, 8, 1, 3, 4, 5, 6, 9, 7};
μ3 = {2, 3, 4, 1};
dSet = Complement[subIndecomposablesOfSet@{π4, π5}, qSetPerms[5, 3, 9]];
showPerms@dSet

```

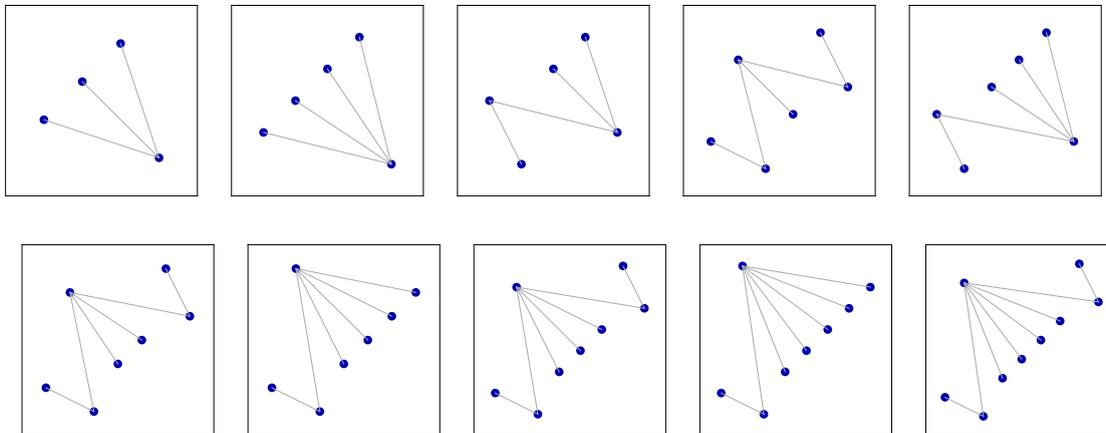

```

q53Seq = countQ[5, 3]
f53Seqs = enumerationsForF[5, 3]
Length@%
downsets[dSet, {μ3}, isSubIndecomp];
dSeqs = sortEnumerations@DeleteDuplicates[enumSeq /@%]
Length@%
addEnumSeqs[addEnumSeqs[q53Seq, buildEnumSeq[First@f53Seqs, 5]], First@dSeqs]
grSumClosed@% // rootForm
N[%, 7]
addEnumSeqs[addEnumSeqs[q53Seq, buildEnumSeq[Last@f53Seqs, 5]], Last@dSeqs]
grSumClosed@% // rootForm
N[%, 7]
{1, 1, 2, 3, 5, 7, 8}

{{1, 1}, {1, 1, 1}, {1, 1, 1, 1}, {1, 2}, {1, 2, 1},
 {1, 2, 1, 1}, {1, 2, 2}, {1, 2, 2, 1}, {1, 2, 2, 2}, {1, 2, 2, 2, 1}}

10
{{0, 0, 0, 1}, {0, 0, 0, 1, 0, 0, 1}, {0, 0, 0, 1, 0, 0, 1, 1}, {0, 0, 0, 1, 0, 1},
 {0, 0, 0, 1, 0, 1, 1}, {0, 0, 0, 1, 0, 1, 1, 1}, {0, 0, 0, 1, 0, 1, 2},
 {0, 0, 0, 1, 0, 1, 2, 1}, {0, 0, 0, 1, 0, 1, 2, 2}, {0, 0, 0, 1, 0, 1, 2, 2, 1},
 {0, 0, 0, 1, 1}, {0, 0, 0, 1, 1, 0, 1}, {0, 0, 0, 1, 1, 0, 1, 1},
 {0, 0, 0, 1, 1, 1}, {0, 0, 0, 1, 1, 1, 1}, {0, 0, 0, 1, 1, 1, 1, 1},
 {0, 0, 0, 1, 1, 1, 2}, {0, 0, 0, 1, 1, 1, 2, 1}, {0, 0, 0, 1, 1, 1, 2, 2},
 {0, 0, 0, 1, 1, 1, 2, 2, 1}, {0, 0, 0, 1, 2}, {0, 0, 0, 1, 2, 0, 1},
 {0, 0, 0, 1, 2, 0, 1, 1}, {0, 0, 0, 1, 2, 1}, {0, 0, 0, 1, 2, 1, 1},
 {0, 0, 0, 1, 2, 1, 1, 1}, {0, 0, 0, 1, 2, 1, 2}, {0, 0, 0, 1, 2, 1, 2, 1},
 {0, 0, 0, 1, 2, 1, 2, 2}, {0, 0, 0, 1, 2, 1, 2, 2, 1}, {0, 0, 0, 1, 2, 2},
 {0, 0, 0, 1, 2, 2, 1}, {0, 0, 0, 1, 2, 2, 1, 1}, {0, 0, 0, 1, 2, 2, 2},
 {0, 0, 0, 1, 2, 2, 2, 1}, {0, 0, 0, 1, 2, 2, 2, 2}, {0, 0, 0, 1, 2, 2, 2, 2, 1}}

37
{1, 1, 2, 4, 5, 7, 9}

rootOf(x^7 - 2 x^6 - x^4 - 2 x^3 - x^2 - 2 x - 2)
2.389038

{1, 1, 2, 4, 7, 9, 11, 12}

rootOf(x^8 - 2 x^7 - x^5 - 2 x^4 - 3 x^3 - 2 x^2 - 2 x - 1)
2.430059

gapInequalities[dSeqs, f53Seqs, 7] // gapIneqsForm
Reduce[And@@% && γ > 1, γ] // rootForm
N[%%[3 ;;], 7]
1 - γ^-2 ≤ γ^-1 + 2 γ^-2 + 2 γ^-3 + γ^-4
γ - 1 - 2 γ^-1 + γ^-2 + γ^-3 ≤ γ^-1 + 2 γ^-2 + 2 γ^-3 + γ^-4
1 - γ^-2 ≤ γ^-1 + 2 γ^-2 + 2 γ^-3 + γ^-4
γ - 1 - 2 γ^-1 + γ^-2 + γ^-3 ≤ γ^-1 + 2 γ^-2 + 2 γ^-3 + γ^-4
γ^2 - γ - 3 - γ^-1 + γ^-2 + 2 γ^-3 + γ^-4 ≤ γ^-1 + 2 γ^-2 + 2 γ^-3 + γ^-4

1 < γ ≤ rootOf(x^4 - 2 x^3 - x^2 - 1)
γ ≤ 2.470979

```

## 4.5 Family E

```

 $\pi_6 = \{3, 4, 1, 2\};$ 
 $\pi_7 = \{2, 6, 1, 3, 4, 7, 5\};$ 
 $\pi_8 = \{3, 1, 4, 5, 6, 8, 2, 7\};$ 
 $\mu_4 = \{2, 3, 4, 5, 1\};$ 
 $\mu_5 = \{2, 3, 5, 1, 4\};$ 
eSet = Complement[subIndecomposablesOfSet@{ $\pi_6, \pi_7, \pi_8$ }, qSetPerms[5, 5, 8]];
showPerms@eSet

```

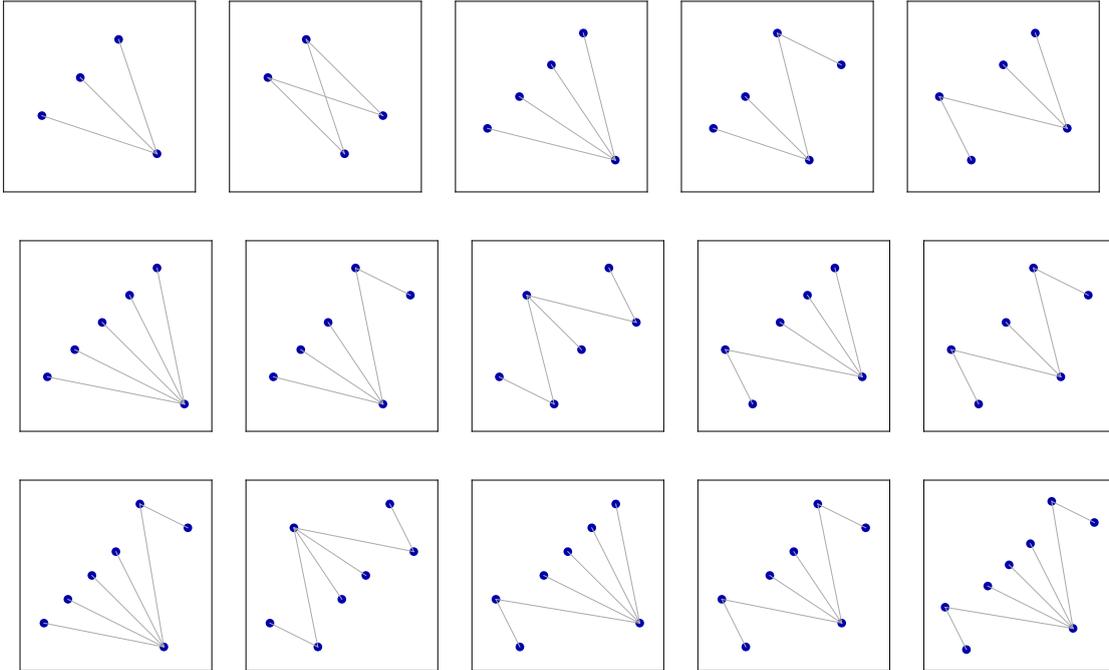

```

q55Seq = countQ[5, 5]
f55Seqs = enumerationsForF[5, 5]
Length@%
Union[downsets[eSet, {π6, μ3}, isSubIndecomp],
      downsets[eSet, {μ2, μ4, μ5}, isSubIndecomp]];
eSeqs = sortEnumerations@DeleteDuplicates[enumSeq/@%]
Length@%
addEnumSeqs[addEnumSeqs[q55Seq, buildEnumSeq[First@f55Seqs, 5]], First@eSeqs]
(grLowerE = grSumClosed@%) // rootForm
N[%, 7]
addEnumSeqs[addEnumSeqs[q55Seq, buildEnumSeq[Last@f55Seqs, 5]], Last@eSeqs]
grUpperE = grSumClosed@% // rootForm
N[%, 7]

```

{1, 1, 2, 3, 5, 7, 9,  $\overline{10}$ }

{1, 1}, {1, 1, 1}, {1, 1, 1, 1}, {1, 2}, {1, 2, 1}, {1, 2, 1, 1}, {1, 2, 2},  
 {1, 2, 2, 1}, {1, 2, 2, 2}, {1, 2, 2, 2, 1}, {1, 2, 3}, {1, 2, 3, 1},  
 {1, 2, 3, 2}, {1, 2, 3, 2, 1}, {1, 2, 3, 3}, {1, 2, 3, 3, 1}, {1, 2, 3, 3, 2},  
 {1, 2, 3, 3, 2, 1}, {1, 2, 3, 4}, {1, 2, 3, 4, 1}, {1, 2, 3, 4, 2}, {1, 2, 3, 4, 2, 1},  
 {1, 2, 3, 4, 3}, {1, 2, 3, 4, 3, 1}, {1, 2, 3, 4, 3, 2}, {1, 2, 3, 4, 3, 2, 1}}

26

{0, 0, 0, 1, 2, 1}, {0, 0, 0, 1, 2, 1, 1}, {0, 0, 0, 1, 2, 2}, {0, 0, 0, 1, 2, 2, 1},  
 {0, 0, 0, 1, 2, 3}, {0, 0, 0, 1, 2, 3, 1}, {0, 0, 0, 1, 2, 3, 2}, {0, 0, 0, 1, 3, 1},  
 {0, 0, 0, 1, 3, 1, 1}, {0, 0, 0, 1, 3, 2}, {0, 0, 0, 1, 3, 2, 1}, {0, 0, 0, 1, 3, 3},  
 {0, 0, 0, 1, 3, 3, 1}, {0, 0, 0, 1, 3, 3, 2}, {0, 0, 0, 1, 3, 4}, {0, 0, 0, 1, 3, 4, 1},  
 {0, 0, 0, 1, 3, 4, 2}, {0, 0, 0, 1, 3, 4, 3}, {0, 0, 0, 1, 3, 5}, {0, 0, 0, 1, 3, 5, 1},  
 {0, 0, 0, 1, 3, 5, 2}, {0, 0, 0, 1, 3, 5, 3}, {0, 0, 0, 1, 3, 5, 3, 1},  
 {0, 0, 0, 1, 3, 5, 4}, {0, 0, 0, 1, 3, 5, 4, 1}, {0, 0, 0, 2}, {0, 0, 0, 2, 0, 1},  
 {0, 0, 0, 2, 0, 1, 1}, {0, 0, 0, 2, 1}, {0, 0, 0, 2, 1, 1}, {0, 0, 0, 2, 1, 1, 1},  
 {0, 0, 0, 2, 1, 2}, {0, 0, 0, 2, 1, 2, 1}, {0, 0, 0, 2, 2}, {0, 0, 0, 2, 2, 1},  
 {0, 0, 0, 2, 2, 1, 1}, {0, 0, 0, 2, 2, 2}, {0, 0, 0, 2, 2, 2, 1}, {0, 0, 0, 2, 2, 3},  
 {0, 0, 0, 2, 2, 3, 1}, {0, 0, 0, 2, 2, 3, 2}, {0, 0, 0, 2, 3}, {0, 0, 0, 2, 3, 1},  
 {0, 0, 0, 2, 3, 1, 1}, {0, 0, 0, 2, 3, 2}, {0, 0, 0, 2, 3, 2, 1}, {0, 0, 0, 2, 3, 3},  
 {0, 0, 0, 2, 3, 3, 1}, {0, 0, 0, 2, 3, 3, 2}, {0, 0, 0, 2, 3, 4}, {0, 0, 0, 2, 3, 4, 1},  
 {0, 0, 0, 2, 3, 4, 2}, {0, 0, 0, 2, 3, 4, 3}, {0, 0, 0, 2, 3, 4, 3, 1},  
 {0, 0, 0, 2, 3, 5}, {0, 0, 0, 2, 3, 5, 1}, {0, 0, 0, 2, 3, 5, 2}, {0, 0, 0, 2, 3, 5, 3},  
 {0, 0, 0, 2, 3, 5, 3, 1}, {0, 0, 0, 2, 3, 5, 4}, {0, 0, 0, 2, 3, 5, 4, 1}}

61

{1, 1, 2, 4, 7, 8, 10,  $\overline{11}$ }

rootOf( $x^8 - 2x^7 - x^5 - 2x^4 - 3x^3 - x^2 - 2x - 1$ )

2.422247

{1, 1, 2, 5, 8, 12, 14, 13, 14, 16, 17,  $\overline{18}$ }

rootOf( $x^{12} - 2x^{11} - x^9 - 3x^8 - 3x^7 - 4x^6 - 2x^5 + x^4 - x^3 - 2x^2 - x - 1$ )

2.485938

While lexicographic ordering suffices for Families A-D, the gap inequalities for family E are very sensitive to the ordering of the enumerations of the extra sets of indecomposables, so we reorder them here by their value at the lower end of the interval of growth rates.

```

eSeqs = SortBy[eSeqs, N[gammaForm[#] /. γ → grLowerE] &];
gapInequalities[eSeqs, f55Seqs, 7] // gapIneqsForm
Reduce[And@@% && γ > 1, γ] // rootForm
N[%, 7]

```

$$1 - \gamma^{-2} \leq \gamma^{-1} + 3\gamma^{-2} + 4\gamma^{-3} + 3\gamma^{-4} + 2\gamma^{-5} + \gamma^{-6}$$

$$\gamma - 1 - 2\gamma^{-1} + \gamma^{-2} + \gamma^{-3} \leq \gamma^{-1} + 3\gamma^{-2} + 4\gamma^{-3} + 3\gamma^{-4} + 2\gamma^{-5} + \gamma^{-6}$$

$$\gamma^3 - 2\gamma^2 - 2\gamma + 2 + \gamma^{-1} \leq \gamma^{-1} + 3\gamma^{-2} + 4\gamma^{-3} + 3\gamma^{-4} + 2\gamma^{-5} + \gamma^{-6}$$

$$-\gamma^3 + 2\gamma^2 + 2\gamma - 1 - \gamma^{-1} - \gamma^{-2} \leq \gamma^{-1} + 3\gamma^{-2} + 4\gamma^{-3} + 3\gamma^{-4} + 2\gamma^{-5} + \gamma^{-6}$$

$$\gamma - 1 - \gamma^{-1} + \gamma^{-2} \leq \gamma^{-1} + 3\gamma^{-2} + 4\gamma^{-3} + 3\gamma^{-4} + 2\gamma^{-5} + \gamma^{-6}$$

$$-\gamma^3 + 2\gamma^2 + 3\gamma - 3 - 2\gamma^{-1} + \gamma^{-2} \leq \gamma^{-1} + 3\gamma^{-2} + 4\gamma^{-3} + 3\gamma^{-4} + 2\gamma^{-5} + \gamma^{-6}$$

$$\gamma^2 - 2\gamma - 2 + 2\gamma^{-1} + \gamma^{-2} \leq \gamma^{-1} + 3\gamma^{-2} + 4\gamma^{-3} + 3\gamma^{-4} + 2\gamma^{-5} + \gamma^{-6}$$

$$-\gamma^3 + \gamma^2 + 4\gamma + 1 - 3\gamma^{-1} - 2\gamma^{-2} \leq \gamma^{-1} + 3\gamma^{-2} + 4\gamma^{-3} + 3\gamma^{-4} + 2\gamma^{-5} + \gamma^{-6}$$

$$\gamma^3 - \gamma^2 - 4\gamma + 3\gamma^{-1} + \gamma^{-2} \leq \gamma^{-1} + 3\gamma^{-2} + 4\gamma^{-3} + 3\gamma^{-4} + 2\gamma^{-5} + \gamma^{-6}$$

$$-\gamma^3 + 6\gamma + 3 - 5\gamma^{-1} - 3\gamma^{-2} \leq \gamma^{-1} + 3\gamma^{-2} + 4\gamma^{-3} + 3\gamma^{-4} + 2\gamma^{-5} + \gamma^{-6}$$

$$\gamma^3 - \gamma^2 - 3\gamma - 2 + \gamma^{-1} + 3\gamma^{-2} + \gamma^{-3} \leq \gamma^{-1} + 3\gamma^{-2} + 4\gamma^{-3} + 3\gamma^{-4} + 2\gamma^{-5} + \gamma^{-6}$$

$$-\gamma^2 + 2\gamma + 3 - 2\gamma^{-1} - 2\gamma^{-2} \leq \gamma^{-1} + 3\gamma^{-2} + 4\gamma^{-3} + 3\gamma^{-4} + 2\gamma^{-5} + \gamma^{-6}$$

$$1 < \gamma \leq \text{rootOf}(x^8 - x^7 - 5x^6 + 2x^5 + 4x^4 + 2x^3 + 2x^2 + x + 1) \vee$$

$$\text{rootOf}(x^8 - 3x^7 + 3x^5 + 2x^3 + 2x^2 + x + 1) \leq \gamma \leq \text{rootOf}(x^6 - 2x^5 - 2x^3 - 2x^2 - x - 1)$$

$$1.000000 < \gamma \leq 1.516475 \quad || \quad 2.363728 \leq \gamma \leq 2.489043$$
